# Supplementary material for: Program Merge Conflict Resolution via Neural Transformers
Source: arXiv:2109.00084 source file (2022-11-29)
Supplement: Supplementary file 1 [file appendix.tex]

\section{Appendix}

\label{sec:appendix}

\subsection{Primitive Merge Resolution Types}
\label{sec:merge_types}

We identify a set of primitive merge resolution patterns based on the analysis of the real-world merge conflict resolutions from GitHub. For a merge tuple $(\mathcal{A}, \mathcal{B}, \mathcal{O}, \mathcal{M})$ with line-level conflicting regions $A_i, B_i, O_i$, i=0...N, and token-level conflicting regions $a^{i}_{j}, b^{i}_{j}, o^{i}_{j}$ corresponding to a line-level conflict $i$, we define following nine basic merge resolution types which serve as labels for supervised classification task:
\begin{enumerate}
\item{Take changes $a^{i}_{j}$ proposed in program $\mathcal{A}$ (developer branch A) as resolution,}
\item{Take changes $b^{i}_{j}$ proposed in program $\mathcal{B}$ as resolution,}
\item{Take code piece $o^{i}_{j}$ in the base reference program $\mathcal{O}$ as resolution,}
\item{Take a string concatenation of changes in $a^{i}_{j}$ and $b^{i}_{j}$ as resolution,}
\item{Take a string concatenation of changes in $b^{i}_{j}$ and $a^{i}_{j}$ as resolution (reverse order as compared to the previous),}
% add REM labels
\item{Take changes $a^{i}_{j}$ proposed in program $\mathcal{A}$, excluding the lines also present in the base reference program $\mathcal{O}$, as resolution,}
\item{Take changes $b^{i}_{j}$ proposed in program $\mathcal{B}$, excluding the lines present in the base, as resolution,}
\item{Take a string concatenation of changes in $a^{i}_{j}$ and $b^{i}_{j}$, excluding the lines present in the base, as resolution,}
\item{Take a string concatenation of changes in $b^{i}_{j}$ and $a^{i}_{j}$, excluding the lines present in the base, as resolution (reverse order as compared to the previous),}
\end{enumerate}
%While the above 9 primitive merge patterns are defined for token-level conflicting chunks, same definition could be applied at line-level, substituting $a^{i}_{j}, b^{i}_{j}, o^{i}_{j}$ chunks with $A_i, B_i, O_i$. 

Our analysis shows that over 99\% of all the merge conflicts can be represented using these labels. While the above nine resolution types are primitive, they form a basis sufficient to cover a large class of real-world merge resolutions in modern version control systems, including arbitrary combinations or interleavings of lines.

%Fig.~\ref{fig:line_labels} shows the label distribution obtained for the standard (line-level) diff3 conflicting regions in our dataset for TypeScript programming language. As seen, nearly 50\% of all cases are trivial -- take changes from branch A or B. Arguably, these cases can be resolved without machine learning and are easily addressed by \textit{take ours} or \textit{take theirs} merge resolution strategies.

Fig.~\ref{fig:token_labels} shows the label distribution obtained for token-level differencing algorithm. It excludes trivial (``take ours'' or ``take theirs'') merge resolutions at line-level. Note, that ``take A'' merge resolution at token-level does not correspond to ``take ours'' or ``take theirs'' merge resolution strategy, and can map to any label at line-level, thus representing a non-trivial merge scenario stimulating for machine learning studies. 

The ``Remove base'' category combines the four primitive merge patterns that remove the lines present in the base branch from the resolution (e.g. take changes proposed in one program and exclude the lines present in base). 
%The ``Other'' category consists of arbitrary line-interleavings. 

%\begin{figure*}
%\begin{center}
%    \includegraphics[width=.75\textwidth]{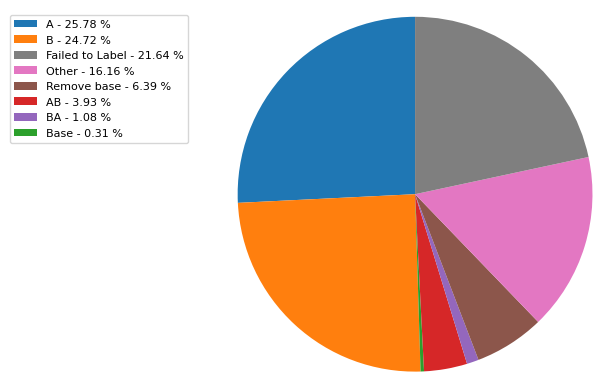}
%\caption{Summary of merge conflict resolution labels in our dataset for TypeScript: label distribution for merge conflicts extracted with the standard (line-level) diff3 algorithm, right. }
%\label{fig:line_labels}
%\end{center}
%\end{figure*}

\begin{figure*}
\begin{center}
    \includegraphics[width=.75\textwidth]{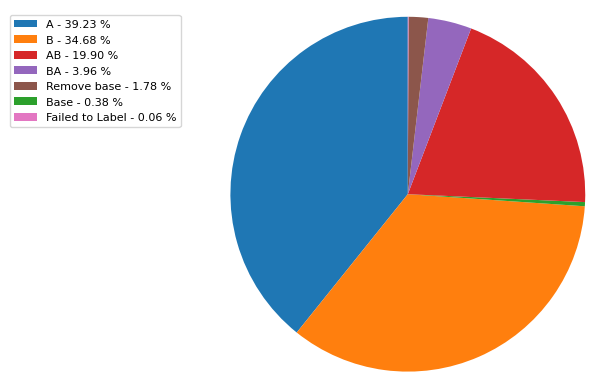}
\caption{Summary of merge conflict resolution labels in our dataset for TypeScript: label distribution for merge conflicts extracted with token-level differencing algorithm. }
\label{fig:token_labels}
\end{center}
\end{figure*}

It is important to stress, these primitive merge resolution types at token-level are not strictly defined \textit{templates} dictating which syntactic structures should be selected from input programs. For instance, a label ``take changes proposed in program $\mathcal{A}$`` can correspond to a single code token as well as an entire method signature or body. As such, the merge types are not restrictive in their representation power of merge conflicts.

\section{Merge Resolution Decoding}
\label{sec:decoding}

Here we provide additional implementation details about the model.

Each model prediction yields a probability distribution \\ $p(r_{j} | a_{j}, b_{j}, o_{j})$ over primitive merge patterns given a token-level conflict. In case of a one-to-many correspondence between original line-level and the token-level conflicts (see, for instance, Fig.~\ref{fig:word_appendix}) to approximate the original $p(R | A, B, O)$ we decode the most promising combination from the predicted solution space. This can be conceptualized as a maximum cost path search on a matrix, which we approach via a beam search algorithm.

\begin{algorithm*}
    \caption{Merge conflict resolution decoding algorithm (beam search) with \thistool{}}\label{alg:decoding}
\begin{algorithmic}
%\State{$R \leftarrow ""$} \Comment{Given a merge tuple $\mathcal{A}$, $\mathcal{B}$, 
%$\mathcal{O}$, $\mathcal{M}$ initialize the resolution to an empty string.}
\State{$b \leftarrow \{r_0, 0\}$} \Comment{Initialize beam \{state, logprob\}}
\State{$\{a_j, b_j, o_j, r_j\}_{j=0...N} \leftarrow \texttt{token_diff3}(\mathcal{A}, \mathcal{B}, \mathcal{O}, \mathcal{M}), $} \Comment{Perform token-level differencing}

%\While{$j < N$} \Comment{For each token-level conflict}
\For{$j \leftarrow 0~ \textbf{to} ~N$}
    %\State{$R \leftarrow pref_j :: R$} \Comment{Update resolution with token-level prefix $j$.}
    \If{$a_j = \emptyset \wedge b_j = \emptyset \wedge o_j = \emptyset$}  \Comment{In case token-level merge results in a clean merge}
    
        \Return $prefix_j :: r_j :: suffix_j$
    \Else
        %\State{$r_j \leftarrow \texttt{mergebert}(a_j, b_j, o_j)$} \Comment{Invoke neural model.}
        \For{$(r_j^{k}, p_j^{k}) \in \textbf{TopK}(\texttt{MergeBERT}(r_{j} | a_{j}, b_{j}, o_{j}))$}
            \State{$b \leftarrow b \cup \{r + prefix_j :: r_j^{k} :: suffix_j, p + p_j^{k}\}$} \Comment{Update beam for each token-level conflict $j$}
        
        \EndFor
        \State{$b \leftarrow \textbf{TopM}(b)$} \Comment{Prune candidates to keep top-M}
        %\State{$R \leftarrow R :: r_j$}
    \EndIf
    %\State{$R \leftarrow pref_j :: R :: suff_j$} \Comment{Update resolution with token-level prefix and suffix $j$.}
\EndFor
\State{$R \leftarrow b[0]$} \Comment{Get resolution region string}
\newline
\Return $R$
\end{algorithmic}
\end{algorithm*}
As a result, the model prediction for each line-level conflict consists of either a label for a token-level conflict or a combination of labels for multiple token-level conflicts representing the best prediction for each token-level conflict within the line-level conflict. Given these labels for each line-level conflict and the contents of the merged file, \thistool{} generates the code corresponding to the resolution region. The contents of the merged file includes the conflict in question and its surrounding regions. Therefore, for each conflicting line, \thistool{} chooses between the versions of code based on the labels the model produced and generates the resolution code by concatenating them. Afterwards, \thistool{} checks the syntax of the generated resolved code, and in case of correctness, outputs it as the candidate merge conflict resolution.

In case of multiple line-level conflicts in the merged file, \thistool{} refines the contents of the merged file that serves as the surrounding region of the conflict. More specifically, for each line-level conflict, \thistool{} replaces the other conflicts in the merged file with the code it previously generated as their predicted resolutions. For this purpose, \thistool{} updates the contents of the merged file after resolving each line-level conflict with the code it generates as the conflict resolution based on the model prediction.

\subsection{Multiple Conflicting Regions}
\label{sec:multiple_regions}

\thistool{} can deal with non-trivial real-world merges, composed of multiple conflicting chunks. To provide an example of such a merge conflict, we include Fig.~\ref{fig:word_appendix}.
\thistool{} correctly predicts a concatenation of changes proposed by developers A and B for the first token-level chunk and a concatenation of changes proposed by developers B and A (in the reverse order) for the second chunk.
\begin{figure*}
    \centering
    \begin{subfigure}[b]{0.5\textwidth}
        \includegraphics[width=\textwidth]{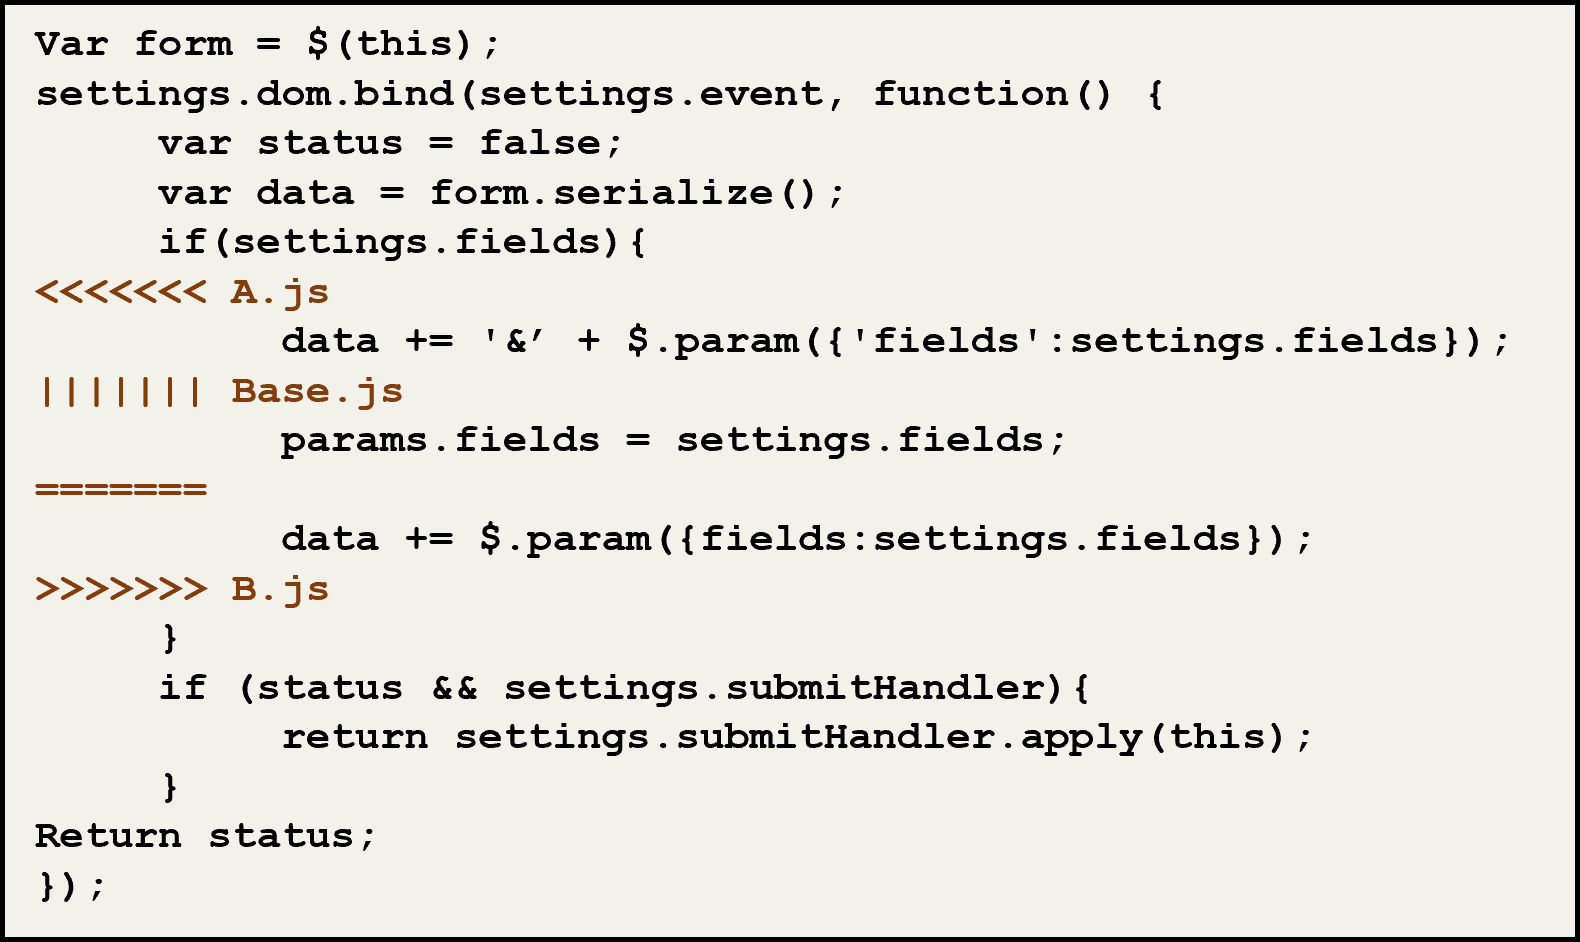}
        \caption{Line-level conflict}
        \label{fig:line-level-conflict-a}
    \end{subfigure}
    \begin{subfigure}[b]{0.5\textwidth}
        \includegraphics[width=\textwidth]{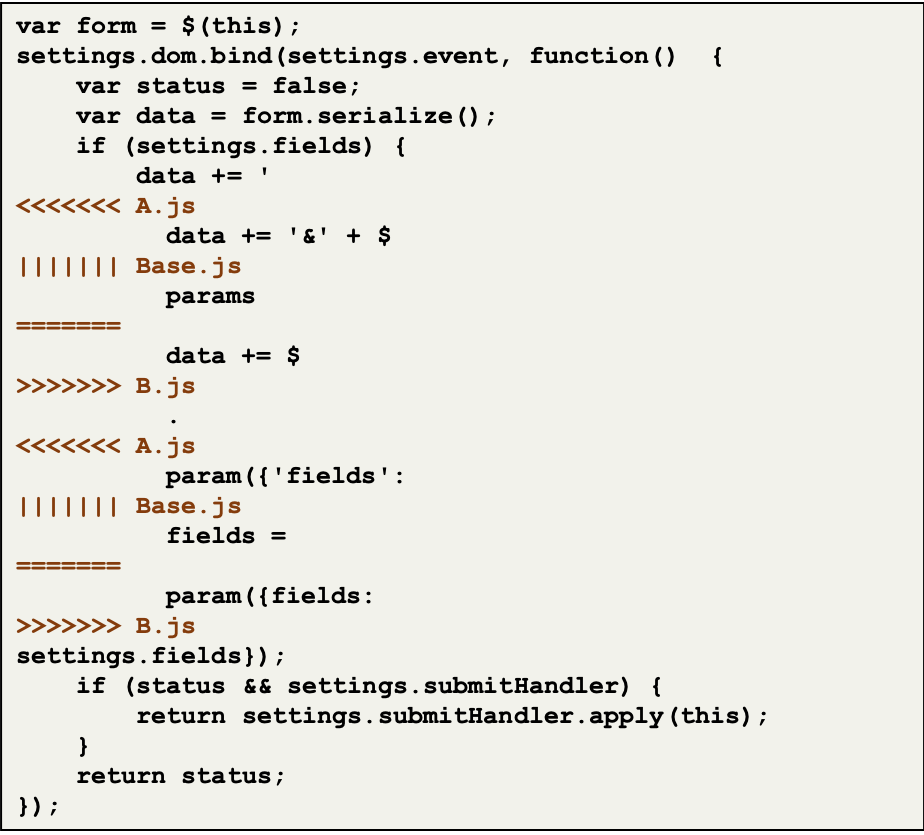}
        \caption{Token-level conflicts}
        \label{fig:token-level-conflict-a}
    \end{subfigure}
    \begin{subfigure}[b]{0.5\textwidth}
        \includegraphics[width=\textwidth]{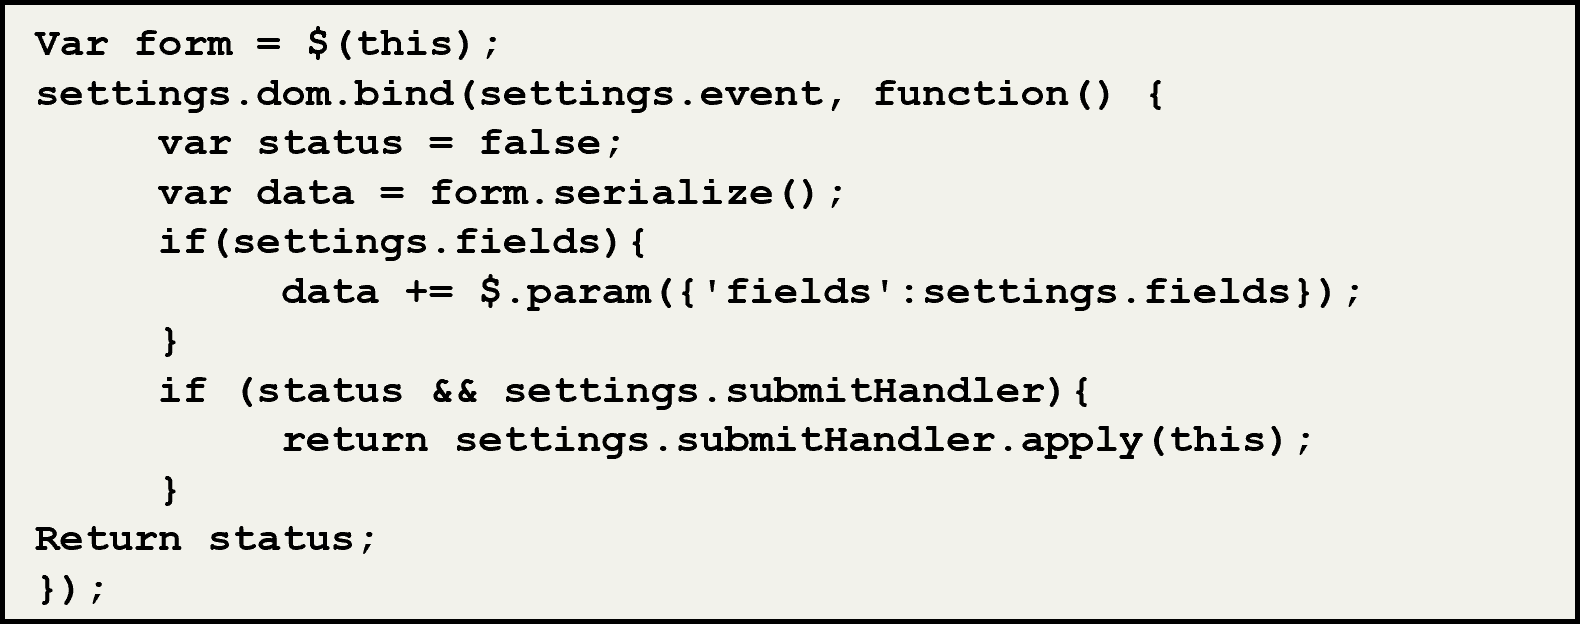}
        \caption{Resolved merge}
        \label{fig:suggested-merge-res-b}
    \end{subfigure}
    \caption{Example real-world merge conflict resolved by \thistool{}. (Top) merge conflict represented through the standard \texttt{diff3}, (middle) corresponding token-level conflicts, and (bottom) the user resolution.}
    \label{fig:word_appendix}
\end{figure*}

\section{User Study Interface}

When a participant opens the interface, the system selects conflicts that the participant has previously resolved and populates the task list with three of them.  Figure 7 show the list of conflicts as tasks for a sample participant.

Once a task is selected, the interface shows a page where they can view the conflict as well as their own resolution and resolution suggestions from MergeBERT.  This is shown in Figure 8.  They can also click on a link to take them to the merge commit in the GitHub repository and explore there if additional context is helpful.

For each resolution suggestion, the authors can indicate if the suggestion is an acceptable merge resolution or not.  Based on their answer to this question, we ask additional followup questions, shown in table 7.  

Participants can choose to skip the conflict and move to the next one if they desire.  Figure 9 shows questions that we ask the participant to answer if they choose to skip a conflict.

\begin{figure*}[th!]
\begin{center}
    \includegraphics[width=.70\textwidth]{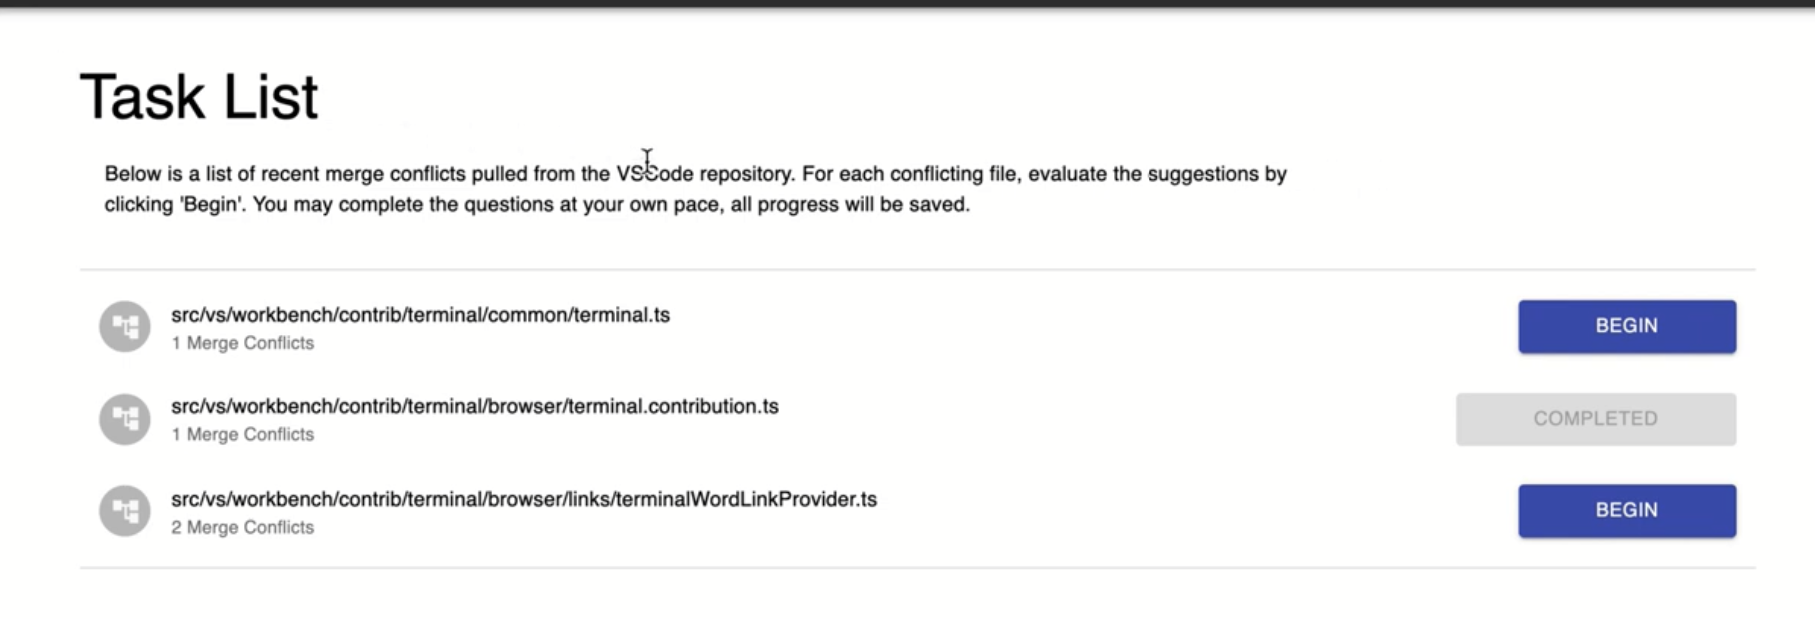}
\caption{This is the main page of the user study interface. Each participant is shown a customized task list, based on merge conflicts they recently resolved.}
\end{center}
\end{figure*}

\begin{figure*}[th!]
\begin{center}
    \includegraphics[width=.75\textwidth]{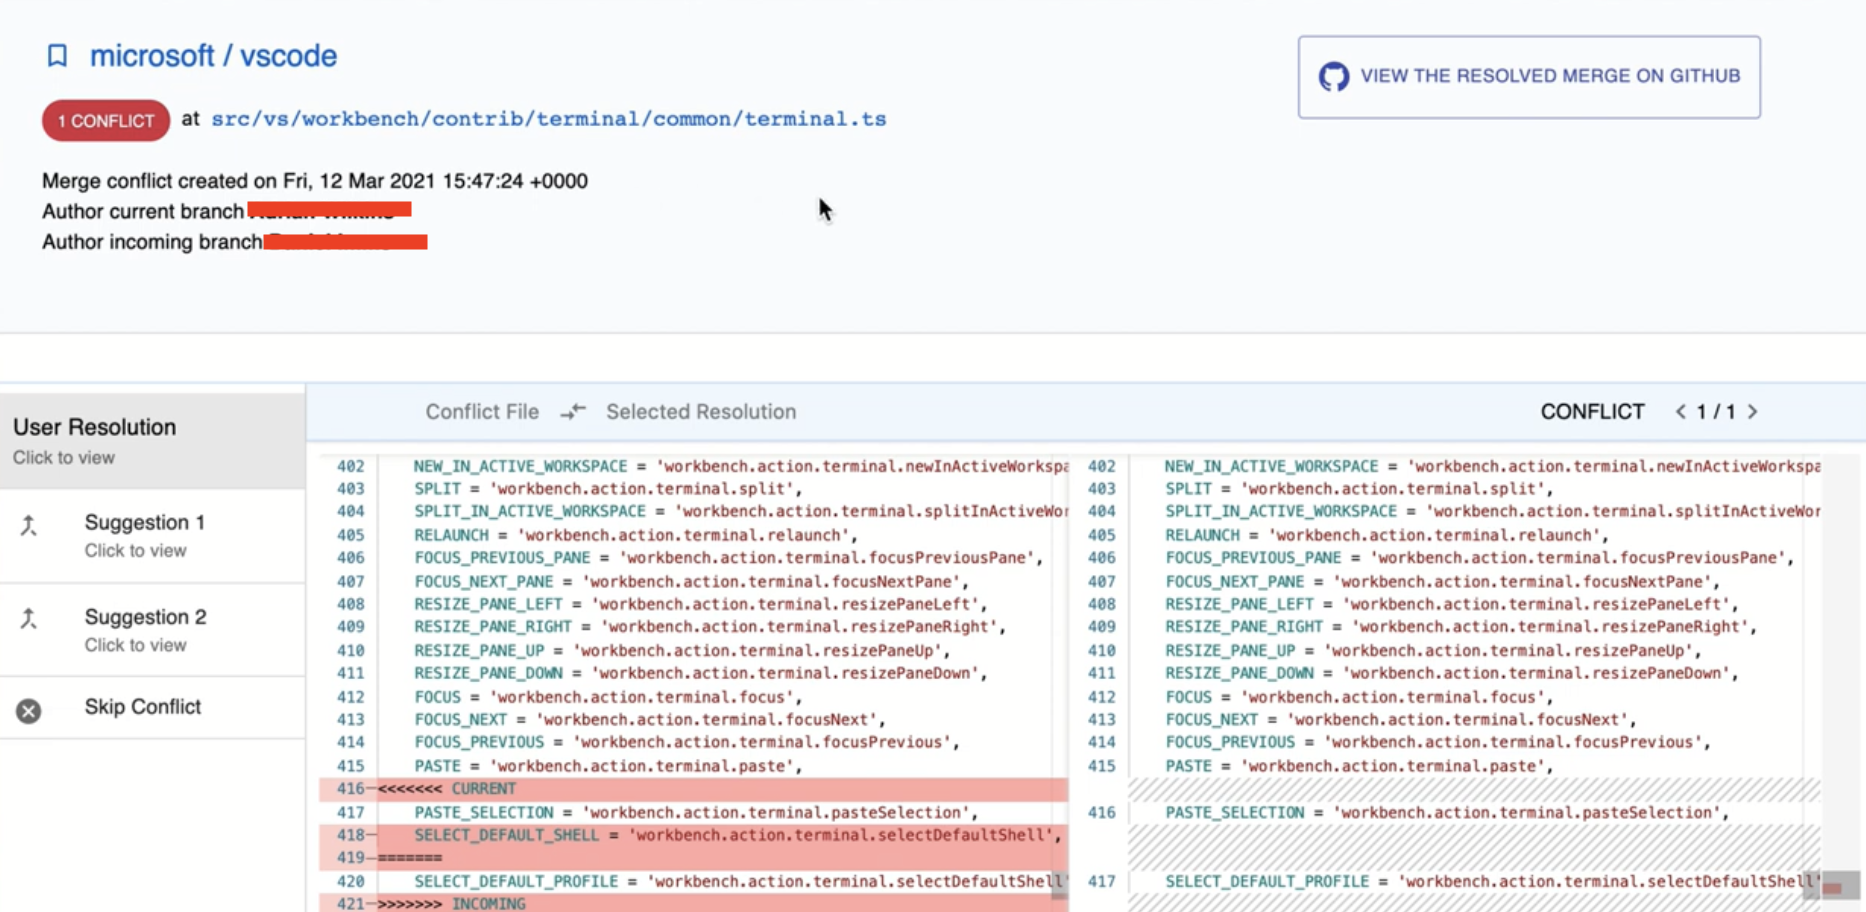}
\caption{After selecting a file from the task list, participants are taken to a page where they can view the conflict file, their original resolution, as well as the resolution suggestions generated by \thistool{}. Participants click on suggestions to evaluate them, or opt to skip a conflict within a file. Participants directly fill out survey questions in a form at the bottom of the page. }
\end{center}
\end{figure*}

\begin{figure*}[th!]
\begin{center}
    \includegraphics[width=.75\textwidth]{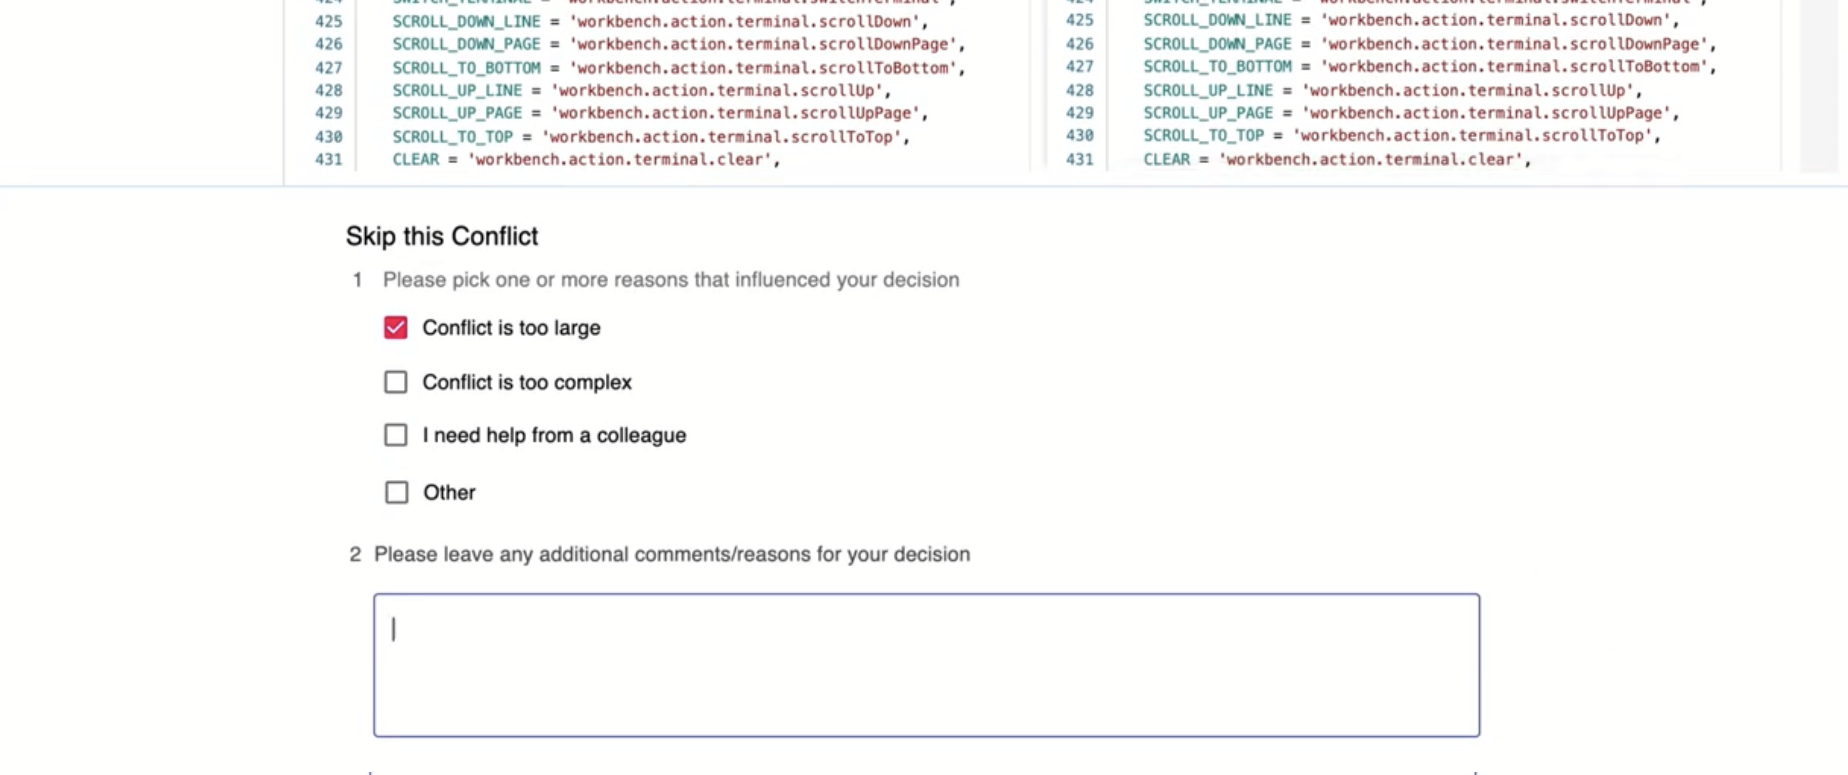}
\caption{Example of questions rendered for the 'Skip Conflict' option. }
\end{center}
\end{figure*}

\begin{table*}[]
\caption{User study questions rendered in the study interface depending on the scenario action taken by the participant. For example, if a participant evaluates a suggestion as 'acceptable' they would answer all questions listed under 'suggestion is acceptable'. }
\begin{tabular}{ll}
\toprule
\textbf{Scenario} & User Study Questions \\ \midrule
Suggestion is acceptable & \begin{tabular}[c]{@{}l@{}}1) Is this suggestion semantically equivalent to the user resolution? \\ 2) Did the order of appearance of different statements play a factor in why you chose this suggestion?\\  3) Open Response\end{tabular} \\ \midrule
Suggestion is not acceptable & \begin{tabular}[c]{@{}l@{}}1) Is any external context needed in order to correctly resolve this conflict? \\ 2) Open response\end{tabular} \\ \midrule
If additional code is added & 1) Is the added code necessary in order to correctly resolve the merge conflict? \\
 \midrule
Skip this conflict & \begin{tabular}[c]{@{}l@{}}1) Multi-select option to explain why\\ 2) Open response \\ 
\end{tabular}
\\ \bottomrule
\end{tabular}
\end{table*}
